# Supplementary material for: Low latency via redundancy
Source: arXiv:1306.3707 source file (2013-06-16)
Supplement: Supplementary file 1 [file appendix-queueing.tex]

%!TEX root = paper.tex
\appendix
\section{Supplement to \S\ref{APPAREF}}
\label{sec:queueing-appendix}

\begin{figure}
\includegraphics[width=0.4\textwidth]{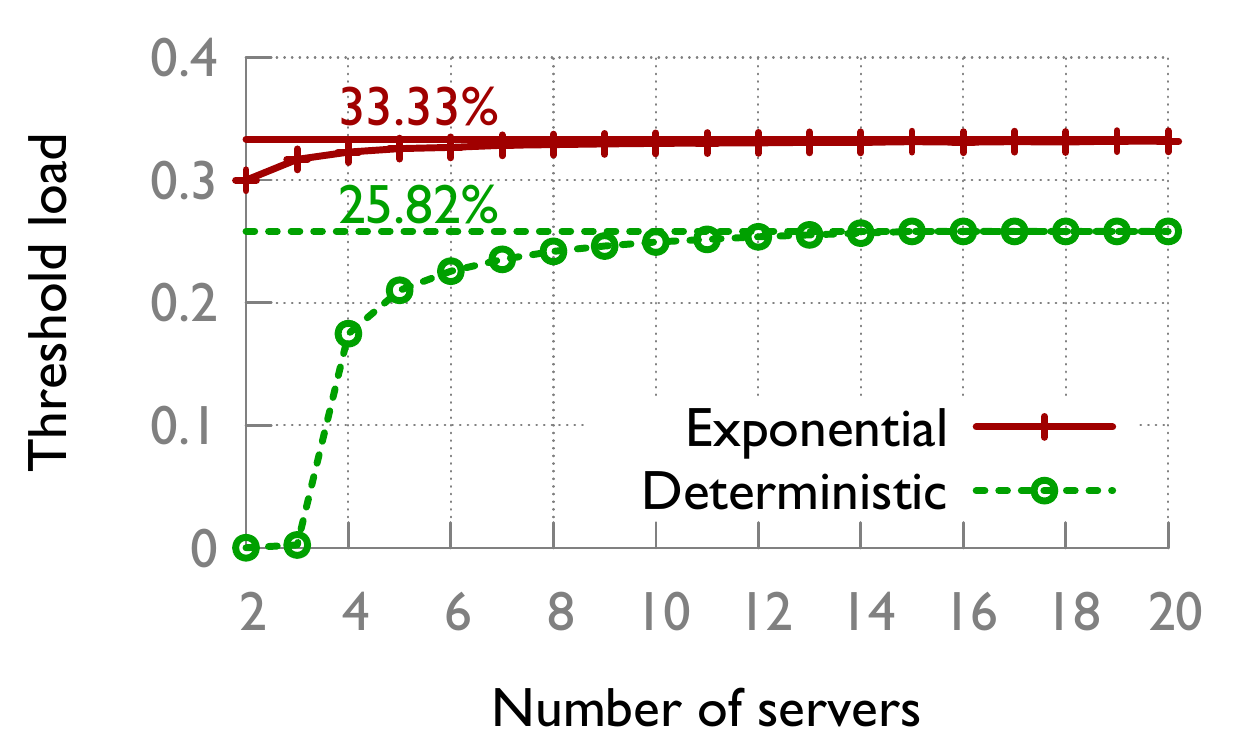}
\caption{Threshold load observed in simulations vs.\ value computed using the independence assumption}
\label{fig:vary-nservers}
\end{figure}

\new{In the analysis in \S\ref{sec:queueing-model}, we made the simplifying assumption that in the steady state, the states of the queues at every server would be completely independent of each other.  This isn't quite accurate because of the correlation in the arrival process.  However, this is a reasonable approximation to make when the number of servers $N$ is much larger than the number of copies $k$ we make of each query.  Figure~\ref{fig:vary-nservers} shows how the threshold load computed using this approximation (analytically in the exponential case, numerically in the deterministic case) compares to the values obtained from simulations of the queueing model.  As the figure shows, the approximation error falls rapidly with $N$.  At $N = 10$, for example, the threshold load with deterministic service time is less than $4\%$ away from the value computed using the approximation.  Note that deterministic service time is the worst case for this approximation: the absence of service variability means that response time is determined entirely by queueing effects.}

\new{We now outline the proofs for the two approximation theorems in \S\ref{sec:queueing-model}.  We omit the details due to space constraints.}

\begin{proof}[of theorem~\ref{thm:myers-vernon} (outline)]
Myers and Vernon~\cite{MyersVernon2012} approximate the queue length distribution (which is a proxy for the response time distribution) by a geometric distribution. The geometric distribution is the discrete analog to the exponential distribution we used in Theorem~\ref{thm:exponential}, and a similar analysis can be used to derive closed form expressions for the mean response time with and without replication as a function of the total load and the variance of the service time distribution. These expressions can then be compared to show that the threshold load has to be smallest when the service time variance is zero --- that is, when the service time distribution is deterministic.
\end{proof}

We note, however, that because of the approximation error involved, using this approximation puts the zero-variance threshold load at about $16\%$, as opposed to the $\approx 25\%$ that we obtain from queueing simulations and numerical calculations.

\begin{proof}[of theorem~\ref{thm:olvera-cravioto} (outline)]
The approximation represents the response time distribution for any given load $\rho$ piecewise, as the combination of an Expo-nential($1$) distribution up to a certain phase-change latency value $\phi(\alpha, \rho)$, and by a heavy-tailed distribution with tail index $\alpha - 1$ for all latencies larger than $\phi(\alpha, \rho)$. Thresholding effects are easy to quantify in the second, heavy-tailed part of the distribution -- for instance, replication always helps performance beyond the $99$th percentile when the base load is $< 44\%$, and it always helps beyond the $92$nd percentile when the base load is $< 30\%$. And when $\alpha < 1 + \sqrt{2}$ it is easy to show that the part of the distribution beyond the $92$nd percentile is responsible for enough of the mass of the entire distribution that the improvement due to redundancy here far outweighs any added cost in the part of the distribution below the $92$nd percentile.
\end{proof}

None of the numbers used in the above analysis --- $30\%$ load, $92$nd percentile, $1 + \sqrt{2}$ --- are very tight. A more careful analysis could likely refine them.

%%% Local Variables: 
%%% mode: latex
%%% TeX-master: "paper"
%%% End: 
